# Supplementary material for: MoFlow: An Invertible Flow Model for Generating Molecular Graphs
Source: arXiv:2006.10137 source file (2020-06-17)
Supplement: Supplementary file 1 [file appendix.tex]

%, implying the potentials to explore large chemical space for drug discovery.

%, which is a flow-based model, to learn invertible mapping between molecular graphs and their latent representations. Our \model generates molecules by first generating bond skeleton through a Glow based model, then generating atoms given bonds by a novel graph conditional flow, and finally combing them into a molecule with postmortem validity correction.

%Our \model has merits of exact and tractable likelihood training, efficient one-pass embedding and generation, chemical validity guarantees, 100\% reconstruction of training data, and good generalization property. We validate our model through four tasks: molecular generation and reconstruction, visualizing continuous latent space, property optimization, and constrained property optimization. Our \model achieves many new state-of-the-art performance, implying the potentials to explore large chemical space for drug discovery.
%  \mytag{Limitations.}   

\section{In Model}
Under the independence assumption for each bond and the conditional independence for each atom given the bonds, the probability of sampling a molecule $M$ from $\mathcal{M}$ is:
\begin{equation}
\begin{aligned}
P_{\mathcal{M}}(M) &= P_{\mathcal{B}}(B) P_{\mathcal{A|B}}(A|B) \\
%&\prod_{i<j} \prod_{l=1}^{c} P_{\mathcal{B}}(B(l, i, j); \theta_{\mathcal{B}})^{B(l,i,j)}  \prod_{i=1}^{n} \prod_{r=1}^{k} P_{\mathcal{A|B}}(A(i, r) | B; \theta_{\mathcal{A|B}})^{A(i,r)} 
&=\prod_{l=1}^{c} \prod_{i<j}^{n\times n}  P_{\theta_\mathcal{B}}(l, i, j)^{B(l,i,j)} \prod_{i=1}^{n} \prod_{r=1}^{k} P_{\theta_\mathcal{A|B}}(i, r | B)^{A(i,r)} 
\end{aligned}
\end{equation}
where $P_{\theta_\mathcal{B}}(l, i, j)$ represents the probability of the bond between atom $i$ and $j$ being type $l$ and $P_{\theta_\mathcal{A|B}}(i, r | B)$ is the conditional probability of the atom $i$ being type $r$ given the bonds $B$. The $\theta_\mathcal{B}$ and $\theta_\mathcal{A|B}$ are learnable modelling parameters. 

\section{Experiments}
\label{sec:app:exp}

We validate our Theorem~\ref{theorem:main}  and the  Corollary~\ref{corollary:main}  together with  parameter inference and simulation algorithms on both synthetic and real-world datasets by answering the following questions:
\bit
\item Can the dynamical systems generate   cross-sectional distributions predicted by our theorem? 

\item Can we learn the parameters of the generated distributions?

\item Can we recover the generative dynamics from its cross-sectional distributions?

\item What are the plausible generative dynamics of a wide range of real-world datasets?

\eit
 %\vspace{-0.05in}
Moreover, to the best of our knowledge, there is no such a theorem serving as our baselines which describies the relationships between a dynamical system and the distribution of its cross-sectional states.
 
\subsection{Synthetic data}
\begin{table}[!htb] % Add the following just after the closing bracket on this line to specify a position for the table on the page: [h], [t], [b] or [p] - these mean: here, top, bottom and on a separate page, respectively
\footnotesize
\centering 
\caption{Experiment Configurations. Generative dynamics and their cross-sectionally generated distributions.}
\begin{tabular}{l c c c c } % The final bracket specifies the number of columns in the table along with left and right borders which are specified using vertical bars (|); each column can be left, right or center-justified using l, r or c. To specify a precise width, use p{width}, e.g. p{5cm}
\toprule % Top horizontal line
%& \multicolumn{3}{c}{\textbf{Net Growth}} & \multicolumn{5}{c}{\textbf{Growth phenomenon}}& \multicolumn{1}{c}{\textbf{Our model}}\\ % Amalgamating several columns into one cell is done using the \multicolumn command as seen on this line
%\cmidrule(l){2-4}   \cmidrule(l){5-9}  \cmidrule(l){10-10}% Horizontal line spanning less than the full width of the table - you can add (r) or (l) just before the opening curly bracket to shorten the rule on the left or right side
 & \makecell{ \textbf{Dynamics}\\ $ \frac{d x_i(t)}{dt}|_{x_0} $ } &  \makecell{\textbf{PDF} \\$ f(x)$}&\textbf{\makecell{Parameters}} \\ % Column names row
\midrule % In-table horizontal line
%\midrule % In-table horizontal line
Exponential & $\frac{1}{\beta t} $& $\beta e^{\beta x}$  &  $\beta = 0.01$\\ % Content row 2
Power Law &  $ \frac{x_i(t) + \Delta}{\alpha t}$   &   $\alpha \Delta^\alpha x^{-(\alpha+1)}$  &\makecell{ $\alpha = 1.5$ \\ $\Delta=1$}\\
\bottomrule 
\end{tabular}
%\caption{Capabilities of models. Only our model meets all specs.} % Table caption, can be commented out if no caption is required
\label{tab:syn_exp} % A label for referencing this table elsewhere, references are used in text as \ref{label}
%\vspace{-0.1in}
\end{table}

% \begin{figure}[!htb]
% %\vspace{-0.1in}
% \centering
% \subfigure[ Exp.  Distribution]{
% \includegraphics[width=0.14\textwidth, trim = 0 0 5 0, clip]{Fig/exp_syn_EXPDist.pdf}
% \label{fig:syn_exp1}
% }
% \subfigure[ Mix.  Generative Dynamics]{
% \includegraphics[width=0.14\textwidth, trim = 0 0 5 0, clip]{Fig/exp_syn_MixDyn.pdf}
% \label{fig:syn_exp6}
% }
% %\vspace{-0.15in}
% \caption{ 
% %\emph{Validation of Theorem~\ref{theorem:main}.} 
% All the  dynamical systems generate cross-sectional samples with predicted distributions. Our model accurately recovers the parameters of these dynamics, and the generators reproduce realistic data samples.  Exp: Exponential, PL:Power-Law, Mix: Mixture. All the figures are on log-log plots.
% \label{fig:syn_exp}}
% %\vspace{-0.2in}
% \end{figure}

\mytag{Experiment setup.} Table~\ref{tab:syn_exp} lists the ground-truth setting with three differential equations to capture three different underlying generative dynamics, whose cross-sectional distribution follows exponential distribution (narrow-tailed), power-law distribution (heavy-tailed), and heavy-tailed mixture distribution respectively predicted by the Theorem~\ref{theorem:main}.  For each dynamical system, we set $E[N(t|\lambda_t)] = 10^6$ agents in the time interval $(0, 10^6]$, namely $\mathscr{P}(t | \lambda_p) = \{t_1, ..., t_i, ...| 0 < t_1 \le...\le t_i \le ..\le t \}$ where $t = 10^6$ and $ \lambda_t=1$. The $10^6$ agents change their states according to dynamics $ \frac{d x_i(t)}{dt}|_{x_0=0}$ as shown in Table~\ref{tab:syn_exp} and we observe their cross-sectional states at time $t = 10^6$.

\mytag{Results.} The dynamics indeed generate cross-sectional observations with predicted distributions by the Theorem~\ref{theorem:main}.
%The cross-sectional observation of the agent states follow the distribution predicted by Theorem~\ref{theorem:main}. 
 As shown in Fig.~\ref{fig:syn_exp} a-c,  the distribution of generated states  (purple dots) fits the ground truth distribution (red lines) exactly for all the model configurations, ranging from  narrow-tailed distribution (Fig.~\ref{fig:syn_exp1}), fat-tailed distribution(Fig.~\ref{fig:syn_exp2}), to mixture of fat-tailed distributions (Fig.~\ref{fig:syn_exp3}).
 
\subsection{Empirical data}
%\vspace{-0.08in}
We examine a wide range of real-world dataset...

% %Appendix A
% \section{Headings in Appendices}
% The rules about hierarchical headings discussed above for
% the body of the article are different in the appendices.
% In the \textbf{appendix} environment, the command

% \begin{acks}
%   The authors would like to thank Dr. Yuhua Li for providing the
%   MATLAB code of the \textit{BEPS} method.

% \end{acks}

Notations in probability theory, survival analysis, point process \cite{aalen2008survival} and dynamical systems /differential equations \cite{barabasi2016network} are used:
\begin{itemize}
\item {\it Probability theory:}
 Let $X$ be a random variable generated from a cumulative distribution function $F(X \le x) = \int^x_{x_0}f(s) ds = 1 - S(X > x)$, and we observe $n$ data samples $x_1$, ..., $x_n$.  Here we assume the $F(X)$ is absolutely continuous.
% and then we generalize the following results to non-absolutely continuous case later.
The $f(x)$ and $S(x) = 1 - F(x)$ are the probability density function  and the survival function (or complementary cumulative distribution function) of the $X$ respectively. 

\item {\it Survival analysis:}
The hazard function $\lambda(x)$ of the $X$ is defined as:
 \begin{equation}
 \footnotesize
\label{equ:hazard}
\lambda(x) = \lim_{\Delta x \to 0^+} \frac{Pr(x \le X < x + \Delta x | X \ge x)}{\Delta x} = \frac{f(x)}{S(x)} \ ,
\end{equation} interpreted as the the probability of $X$ sampled with  value $x^+$ conditional on $X$ not being sampled with value smaller than $x$. 
We define $\Lambda(x) = \int^x_{x_0}\lambda(s) ds$ as the cumulative hazard function. Due to the fact that $\Lambda(x)$ is monotonically increasing, thus $\Lambda(x)$ is invertable and we define $\Lambda^{-1} : \mathscr{R^+} \to \mathscr{R} $, $ \Lambda^{-1}(\Lambda(x)) = x$.  Similarly, we can define  $F^{-1} : \mathscr{R^+} \to \mathscr{R} $, $ F^{-1}(F(x)) = x$.
\item {\it Point process:}
We use $\mathscr{P}(t | \lambda_p) = \{t_1, ..., t_i, ...| 0 < t_1 \le...\le t_i \le ..\le t \}$ to denote a   Poisson point process until time $t$ with the occurrence time $t_i$ of event $i$,  and intensity rate $\lambda_p > 0$.  
\end{itemize}

\subsection{Proposed Theorem and Corollary}
%\mytag{The Theorem and Corollary.} 
Our main theorem  gives the generative dynamics of an arbitrary distribution function $F(x)$  as follows:
%(We defer proofs to the Sec.\ref{sec:si_proof} in \SI):
%{\em \SI \ Sec. The Proof.}): 
\begin{theorem}\label{theorem:main}
%Given a dynamical system $\mathscr{D}(t) = \{x_i(t)| \frac{d x_i(t)}{dt}; x_i{(t_i)} = x_0; i = 1, 2, ... \}$, whose  agents' arriving time  $\{t_1, ..., t_i,....| t_1 \le...\le t_i \le ..\le t \}$ follow a Poisson process $\mathscr{P}(t | \lambda_p)$  ,   and the states  are determined by dynamics $\frac{d x_i(t)}{dt} = \frac{d \Lambda ^{-1} (\ln (\frac{S(x_0)}{t_i} t))}{dt}$ with initial state $x_0$, then a cross-sectional state of $\mathscr{D}(t)$ at time $t$, namely, $ \{x_1(t ), ...,  x_i(t),... \}$, follows distribution $F(x(t))$.
Given a dynamical system $\mathscr{D}(t) = \{x_i(t) > 0| \frac{d x_i(t)}{dt}, \\ x_i{(t_i)} = x_0; i = 1, 2, ... \}$ consisting of agent $i$ who arrives in the system at time $t_i$ according to a Poisson process $\mathscr{P}(t | \lambda_p) = \{t_1, ..., t_i,....| 0 < t_1 \le...\le t_i \le ... \le t \}$ ,  the state of agent $i$  changes according to a differential equation $\frac{d x_i(t)}{dt}|_{x_0}$ with initial value $x_0$, and the cross-sectional states of $\mathscr{D}(t)$ at time point $t$, namely  $ x(t) =  \{x_1(t ), ...,  x_i(t),... \}$, follows the distribution $F(x(t))$ if and only if  $\ \frac{d x_i(t)}{dt}|_{x_0} = \frac{d F^{-1}(1-\frac{t_i}{t})}{dt}$.
%=\frac{d \Lambda ^{-1} (\ln (\frac{S(x_0)}{t_i} t))}{dt}$.
\end{theorem}

\subsection{Proof}
\label{sec:app:si_proof}
 
\begin{lemma}\label{lemma:poisson} \cite{daley2003introduction}
Given a Poisson process $\mathscr{P}(t | \lambda_p) = \{t_1, ..., t_i, ...| 0< t_1 \le...\le t_i \le ..\le t \}$  with $N(t|\lambda_t) = n$, then the probability density function of a random event time $t_i$ given the total time $t$ is $f(t_i) = \frac{1}{t}$,  indicating a uniform distribution on $(0, t]$.
\end{lemma}
\begin{proof}
The joint probability density function of random variables $t_i, i = 1, ..., n $ is:
 \begin{equation}
  \footnotesize
\begin{aligned}
\label{equ:poissonuni} %\lim _{\delta_i \to 0, i = 1, ..., n} 
&Pr(t_i < T_i \le t_i + \delta_i, i = 1, ..., n | N(t) = n) = \\
&\left[\dfrac{\splitdfrac{Pr(N(t_i + \delta_i) -  N(t_i) = 1, N(t_{j+1}) - N(t_{j} + \delta_{j}) = 0, 
}{i = 1,...,n, j = 0, ...,n, t_0 = 0, \delta_0 = 0) }}
{Pr( N(t) = n)}\right]\\
&= \frac{\prod_{i = 1}^{n} \lambda_p \delta_i e^{-\lambda_p \delta_i} e^{-\lambda_p (t-\sum_{i=1}^{n}\delta_i)}}{e^{-\lambda_p t }(\lambda_p t)^n / n!} = \frac{n!}{t^n} \prod_{i = 1}^{n} \delta_i,
%f(x|\theta=1) & = \lambda(x|\theta=1)e^{-\int_{0}^x \lambda(s|\theta=1) ds} \\
%&= (\beta + \frac{\alpha}{x+\Delta}) e^{-\beta x - \alpha \ln (\frac{x}{\Delta}+1)}\\
%&= \beta e^{-\beta x} (\frac{x}{\Delta}+1)^{-\alpha} + \frac{\alpha}{\Delta} (\frac{x}{\Delta} + 1)^{-(\alpha+1)}e^{-\beta x}
\end{aligned}
\end{equation}
 and thus:
 \begin{equation}
  \footnotesize
\begin{aligned}
\label{equ:poissonuni} %\lim _{\delta_i \to 0, i = 1, ..., n} 
&f(t_i, i = 1, ..., n | N(t) = n) \\
&= \lim _{t_i \to 0, i = 1,...,n} \frac{Pr(t_i < T_i \le t_i + \delta_i, i = 1, ..., n | N(t) = n) }{\prod_{i = 1}^{n} \delta_i} \\
 &= \frac{n!}{t^n},      \\
%f(x|\theta=1) & = \lambda(x|\theta=1)e^{-\int_{0}^x \lambda(s|\theta=1) ds} \\
%&= (\beta + \frac{\alpha}{x+\Delta}) e^{-\beta x - \alpha \ln (\frac{x}{\Delta}+1)}\\
%&= \beta e^{-\beta x} (\frac{x}{\Delta}+1)^{-\alpha} + \frac{\alpha}{\Delta} (\frac{x}{\Delta} + 1)^{-(\alpha+1)}e^{-\beta x}
\end{aligned}
\end{equation} where $0 < t_1 \le ...\le ti \le ... \le t$. For the order statistics $t_i, i = 1, ..., n$, $f(t_i) = \frac{1}{t}$.
\end{proof}

\begin{table*}[!htb] 
% \footnotesize
%\vspace{-0.2in}
%\tiny
\centering % Centers the table on the page, comment out to left-justify
\caption{Generative performance on QM9}
\begin{tabular}{l c c c c c c c} % The final bracket specifies the number of columns in the table along with left and right borders which are specified using vertical bars (|); each column can be left, right or center-justified using l, r or c. To specify a precise width, use p{width}, e.g. p{5cm}
\toprule % Top horizontal line
%& \multicolumn{3}{c}{\textbf{Net Growth}} & \multicolumn{5}{c}{\textbf{Growth phenomenon}}& \multicolumn{1}{c}{\textbf{Our model}}\\ % Amalgamating several columns into one cell is done using the \multicolumn command as seen on this line
%\cmidrule(l){2-4}   \cmidrule(l){5-9}  \cmidrule(l){10-10}% Horizontal line spanning less than the full width of the table - you can add (r) or (l) just before the opening curly bracket to shorten the rule on the left or right side
 & \textbf{\% Validity} &  \textbf{\% Novelty} & \textbf{\% Uniqueness} & \textbf{\% Reconstruct} &  \textbf{\% N.U.V.} & \textbf{\% Uniqueness2} \\ % Column names row
\midrule % In-table horizontal line
%\midrule % In-table horizontal line
\textbf{MoFlow} & $96.04\pm0.45$ & $98.39\pm0.24$  &  $98.42\pm0.29$ &$100$  & $93.00\pm0.43$& $94.52\pm0.49$\\ 
\textbf{GraphNVP} & $83.1\pm0.5$ & $58.2\pm1.9$  &  $99.2\pm0.3$ &$100$ & $47.97$& $82.43$\\ 
\bottomrule 
\end{tabular}
%\caption{Capabilities of models. Only our model meets all specs.} % Table caption, can be commented out if no caption is required
\label{tab:app:qm9} % A label for referencing this table elsewhere, references are used in text as \ref{label}
%\vspace{-0.1in}
\end{table*}
